# Supplementary material for: ReMatch: Retrieval Enhanced Schema Matching with LLMs
Source: arXiv:2403.01567 source file (2024-05-30)
Supplement: Supplementary file 1 [file appendix.tex]

\section{Full Matching Prompt}
\label{appendix: full matching prompt}
\subsection{Prompt}

\textit{You are an expert in databases, and schema matching at top k specifically. Your task is to create matches between source and target tables and attributes. For each attribute from the source you always suggest the top 2 most relevant tables and columns from the target. You are excellent at this task.\\
If none of the columns are relevant,  the last table and column should be "NA", "NA". This value may appear only once per mapping!\\
Your job is to match the schemas. You never provide explanations, code or anything else, only results.
Below are the two schemas.\\
Create top k matches between source and target tables and columns.\\
Make sure to match the entire input. Make sure to return the results in the following json format with top 2 target results foreach input in source.\\}

\noindent Expected output format:\\
\texttt{\{'1': \{'SRC\_ENT': 'SOURCE\_TABLE\_NAME', 'SRC\_ATT': 'SOURCE\_COLUMN\_NAME', \\
	   'TGT\_ENT1': 'TARGET\_TABLE\_NAME1', 'TGT\_ATT1': 'TARGET\_COLUMN\_NAME1', 
	   'TGT\_ENT2': 'TARGET\_TABLE\_NAME2', 'TGT\_ATT2': 'TARGET\_COLUMN\_NAME2'\},\\ 
 '2': \{'SRC\_ENT': 'SOURCE\_TABLE\_NAME', 'SRC\_ATT': 'SOURCE\_COLUMN\_NAME',\\
	   'TGT\_ENT1': 'TARGET\_TABLE\_NAME1', 'TGT\_ATT1': 'TARGET\_COLUMN\_NAME1',
	   'TGT\_ENT2': 'TARGET\_TABLE\_NAME2', 'TGT\_ATT2': 'TARGET\_COLUMN\_NAME2'\}\} }...\\
 
\noindent Source Schema:\\
\texttt{,SRC\_ENT, SRC\_ATT \\
0,ADMISSIONS, SUBJECT\_ID\\
1,ADMISSIONS, HADM\_ID} \\
\[\#\#\#\texttt{16 more rows}\#\#\#\]

\noindent ADMISSIONS\\
The ADMISSIONS table gives information regarding a patient's admission to the hospital.\\
Primary Keys:\\
HADM\_ID (INTEGER): Each row of this table contains a unique HADM\_ID, which represents a single patient's admission to the hospital. HADM\_ID ranges from 1000000 - 1999999.\\
Foreign Keys:\\
SUBJECT\_ID (INTEGER): The ADMISSIONS table can be linked to the PATIENTS table using SUBJECT\_ID. References to [PATIENTS, SUBJECT\_ID]\\
Other Columns:\\
ADMITTIME (TIMESTAMP): provides the date and time the patient was admitted to the hospital
\[\#\#\#\texttt{15 more rows}\#\#\#\]

\noindent Target Schema:\\
\texttt{,TGT\_ENT,TGT\_ATT\\
0,PERSON,person\_id\\
1,PERSON,gender\_concept\_id\\
\[\#\#\#\texttt{17 more rows}\#\#\#\]
19,VISIT\_OCCURRENCE,visit\_occurrence\_id\\
20,VISIT\_OCCURRENCE,person\_id}\\
\[\#\#\#\texttt{38 more rows listing all retrieved target tables}\#\#\#\]

\noindent PERSON\\
This table serves as the central identity management for all Persons in the database. It contains records that uniquely identify each person or patient, and some demographic information.\\
Primary Keys:\\
person\_id (bigint): It is assumed that every person with a different unique identifier is in fact a different person and should be treated independently.\\
Foreign Keys:\\
gender\_concept\_id (integer): This field is meant to capture the biological sex at birth of the Person. This field should not be used to study gender identity issues. References to [CONCEPT, concept\_id]\\
\[\#\#\#\texttt{76 more rows describing all target tables}\#\#\#\]

\noindent \textit{Remember to match the entire input. Make sure to return only the results!}

\subsection{GPT-4 Hyperparameters}
The model version used for generation was GPT-4-1106, with the following settings:\\
\texttt{\{seed=42
      temperature=0.5,
      max\_tokens=4096,
      top\_p=0.9,
      frequency\_penalty=0,
      presence\_penalty=0\}}
